# Supplementary material for: Pix2Surf: Learning Parametric 3D Surface Models of Objects from Images
Source: arXiv:2008.07760 source file (2020-08-18)
Supplement: Supplementary file 1 [file comparisons.tex]

\Image{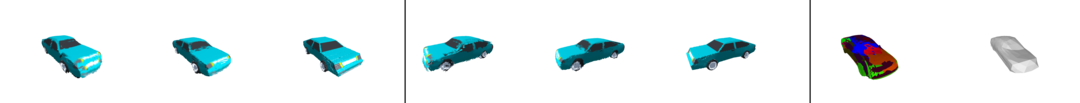}
\Image{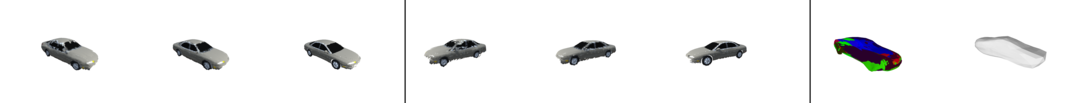}
\Image{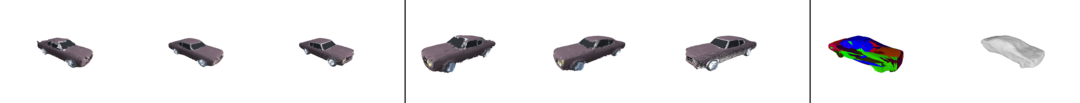}
\Image{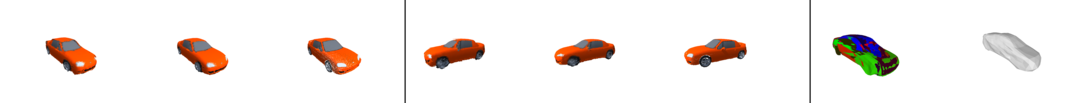}
\Image{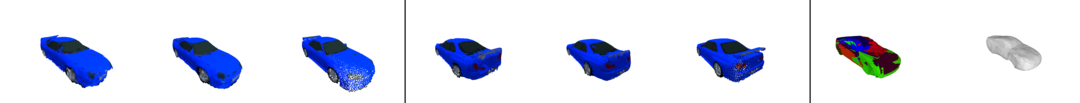}
\Image{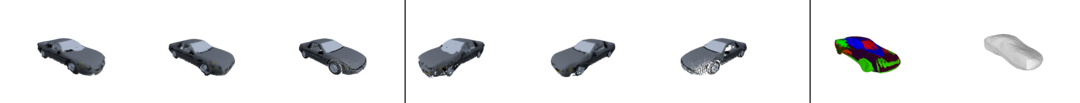}
\Image{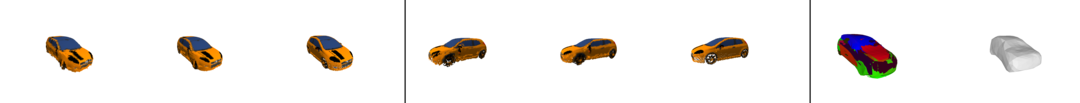}
\Image{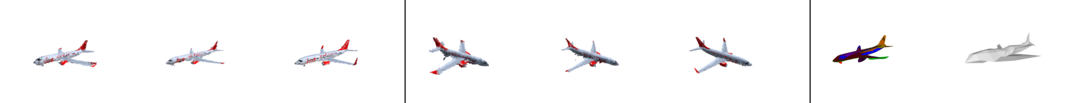}
\Image{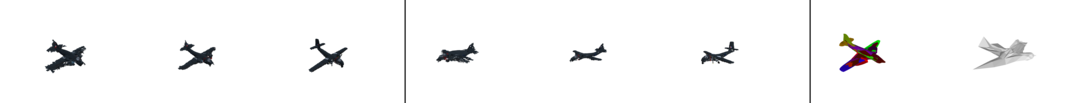}
\Image{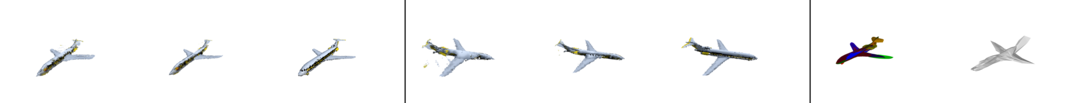}
\Image{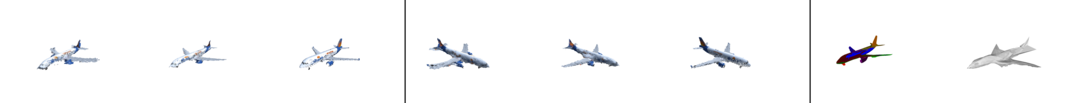}
\Image{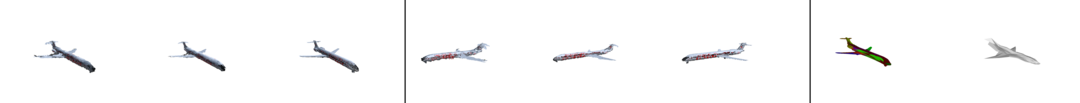}
\Image{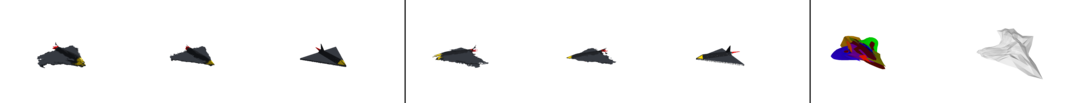}
\Image{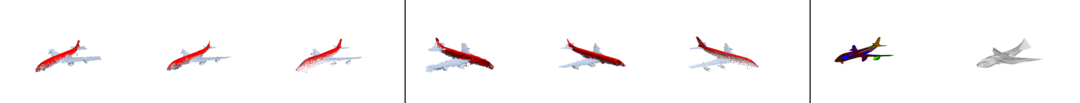}
\Image{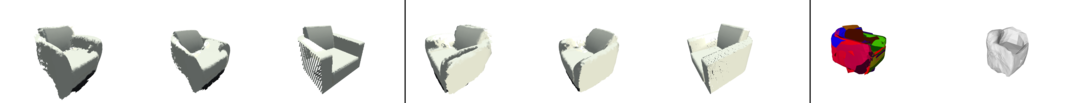}
\Image{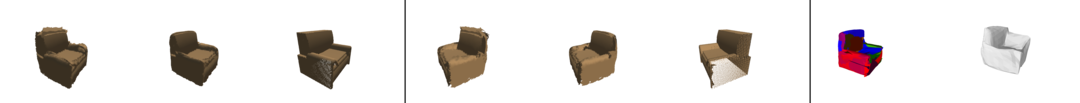}
\Image{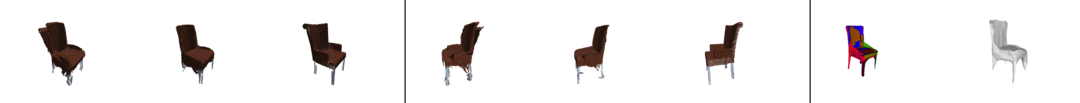}
\Image{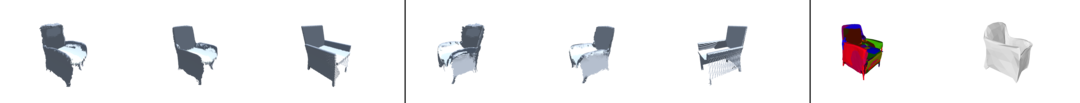}
\Image{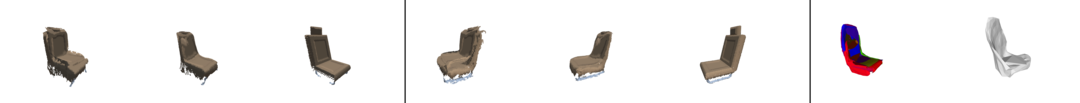}
\Image{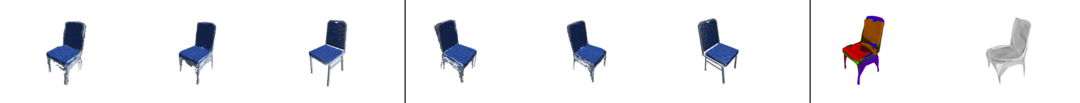}
\Image{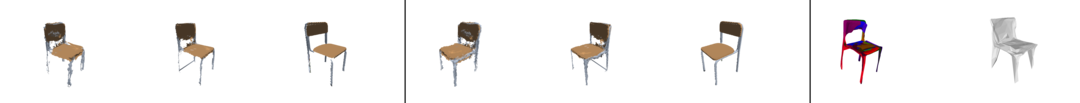}
